# Supplementary material for: One Wide Feedforward is All You Need
Source: arXiv:2309.01826 source file (2023-10-21)
Supplement: Supplementary file 1 [file ablations.tex]

\subsection{Reducing FFN dimension}
\label{app:reducing-ffn-dimension}
We analyze the effect of reducing the FFN dimension of a baseline model ($d_{ff}$) in the encoder (\textcolor{red}{red}) and the decoder (black) from $4096$ down to $0$ in \Cref{fig:ffndim_sweep}. 
As expected, accuracy decreases as we reduce the $d_{ff}$. 
Interestingly, we observe a different trend between encoder and decoder where the decoder is significantly less sensitive to reduction of $d_{ff}$ than the encoder.
\telmo{I think we can remove this. Not adding much.}

\begin{figure}[t]
    \centering
    \includegraphics[width=\columnwidth]{Figures/ffndim_sweep.pdf}
    \caption{Effect of changing the FFN dimension on the Transformer Big for \len$\rightarrow$\lde.}
    \label{fig:ffndim_sweep}
    %\telmo[inline]{Yes, hard to read. I need to figure this one out.}
\end{figure}
